# Supplementary material for: Application of Information Centric Networking to NoSQL Databases: the Spatio-Temporal use case
Source: arXiv:1703.06348 source file (2017-03-18)
Supplement: Supplementary file 1 [file appendix.tex]

\section*{APPENDIX I - Indexing Design-old}
A key design choice of a spatial database is how to map the space in an internal data structure to improve the speed of spatial operations. The mapping strategy is known as indexing method. In general, an indexing method partitions the space in regions that can be further decomposed in sub-regions. The resulting region hierarchy forms a tree data structure. Most popular indexing methods are Grid, R-Tree, and their variants \cite{MicrosoftSQL}.
 
Grid methods decompose the space into a uniform grid. A region of the grid, called \emph{tile}, can be iteratively split into smaller tiles, realizing a multi-layer hierarchical grid structure. Tiles are the nodes of the tree indexing structure \cite{quadtree}. Range-queries can be carried out "tessellating" the requested window with grid tiles and then fetching tiles data. 

R-trees decompose the space in overlapping rectangles \cite{guttman1984r}, whose number, size and position depend on the stored spatial objects. Spatial objects are enclosed in rectangles, each rectangle is a node of the indexing tree and it is the minimum bounding rectangle that encloses its child rectangles; leaf rectangles contain only one spatial object. A range-query is carried out using a recursive algorithm: starting from the root node it go down in the tree.  

The general methodology we follow to realize an ICN distributed spatial database consists in assigning unique and routable name prefixes to the regions identified by the indexing process. Fig. \ref{f:grid} reports an example of such regions (R) in case of Grid and R-tree indexing schemes and point objects. Each database engine stores data of a subset of regions and exposes the region name-prefixes to the ICN routing plane. Such a solution can be applied both in case of Grid and R-tree indexing. However, OpenGeoBase uses a Grid index, as we believe that it is better suited to work with ICN. Indeed: 

\begin{itemize}
	\item regions of a Grid index do not change, i.e., do not depend on the stored objects. Thus, we can assign unique name-prefixes to them at the system roll-out, and ICN routing updates will be needed only in case of administrative reconfigurations, e.g. moving region data from an engine to another one. If regions were dynamic, like in the case of R-Tree, we would risk the introduction of new names in the system and routing plane updates at each data insert or removal;
	\item nodes of a Grid indexing tree have a unique parent node, easing the use of hierarchical naming schemes. In case of R-tree, a node of the index may have multiple parents and parents may change over time, thus complicating the use of a hierarchical naming scheme;	
	\item query-handler and insert-handler need to know the shape of regions, to resolve which are the regions involved in range-query and data insert operations. Such knowledge is implicit for Grid methods, and resolution can be autonomously performed by end-devices or application servers. In R-tree methods, the region shape is not known a-priori and can change; thus, the resolution algorithm needs to be either informed of changes, or realized in recursive way \cite{du2007sd}, so increasing the number of message exchanges involved in the resolution process and then the query time.
\end{itemize}

\begin{figure}[t]
	\centering
	\subfigure[Grid]{  
		\includegraphics[scale=0.30]{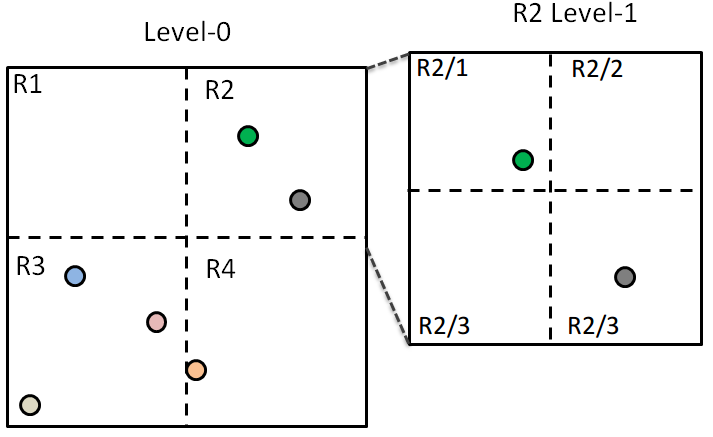}
		\label{f:grid}
	}
	\subfigure[R-tree]{  
		\includegraphics[scale=0.30]{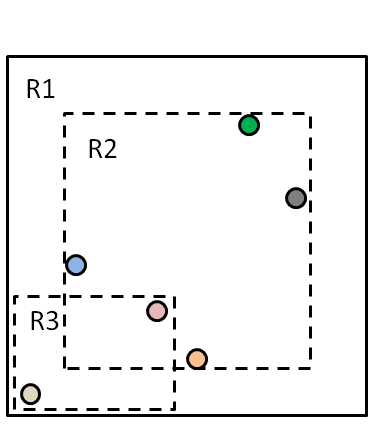}
		\label{f:rtree}
	}
	\caption{Regions of Grid and R-tree indexing schemes}
	%\label{f:indexing}
	
\end{figure}

\section*{APPENDIX II - Database Engine Internal Design}

A database engine processes tile-queries expressed by means of Interests of OGB-Tile contents, and stores geo-referenced data in the form of OGB-Data ContentObjects. To construct the engine, we extend the NDN Repo-ng \cite{ndn}. Repo-ng is formed by: a front-end module that processes Interest messages and TCP bulk-inserts; a back-end database management system (DBMS), in which it is possible to SELECT and INSERT ContentObjects through SQL transactions. The DBMS of NDN Repo-ng is SQLite and contains a single table (CO-Table), whose rows are the stored ContentObjects. 

We extend Repo-ng in order to handle and speed up the processing of tile-queries. We add three tables to the DBMS, named Tile-Tables, one for each OpenGeoBase spatial grid level. The rows of the level-$n$ Tile-Table contain the names of OGB-Data ContentObjects belonging to any tile of level-$n$. When a tile-query for a tile $x$ of level-$n$ is received, the front-end performs an SQL SELECT on the rows of level-$n$ tile-table, searching for names whose prefix is equal to the prefix of tile $x$. By having different tables per level, we reduce the search space and the tile-query processing time. Clearly, other possible table designs are possible, but here we wish to put forward the problem, rather than finding the best solution. The SQL SELECT returns to the Repo-ng front-end the names of ContentObjects, which are retrieved from the CO-Table. The Repo-ng front-end collects and sends them back to the querying devices, within one or more OGB-Tile ContentObjects, by using plain NDN segmentation. 
We also modify the Repo-ng TCP-bulk-insert procedure, so as to create related rows of tile-tables.

\begin{figure*}[t]
	\centering
	\subfigure[Range-query (pink box)]{ 
		\includegraphics[scale=0.26]{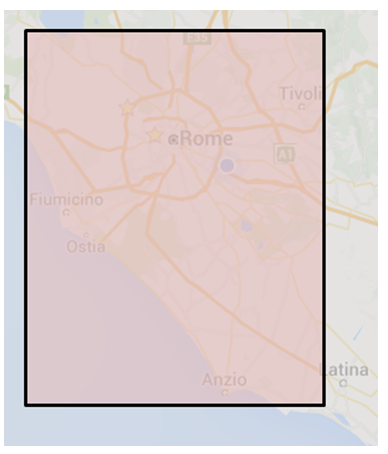}
		\label{f:range-query}
		
	}
	\subfigure[Min stretch tessellation]{ 
		\includegraphics[scale=0.26]{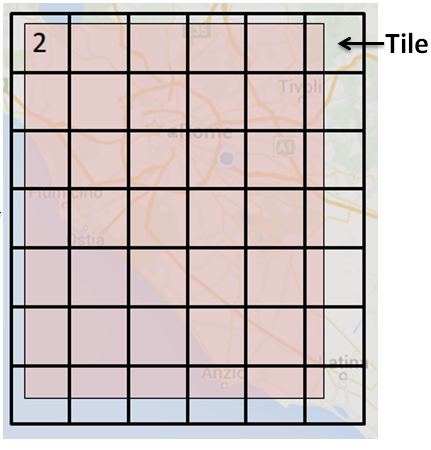}
		\label{f:min-streatch}
		
	}
	\subfigure[Min stretch-and-tiles tessellation]{ 
		\includegraphics[scale=0.26]{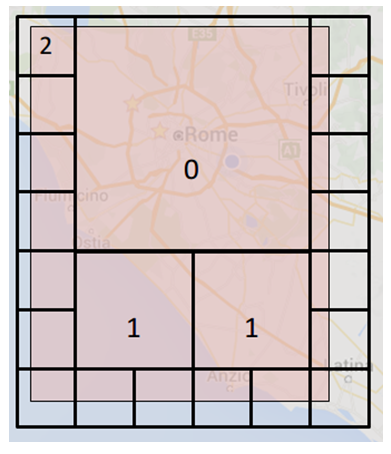}
		\label{f:min-streatch-and-tiles}
		
	}
	\subfigure[Constrained tessellation ($k=19$)]{ 
		\includegraphics[scale=0.26]{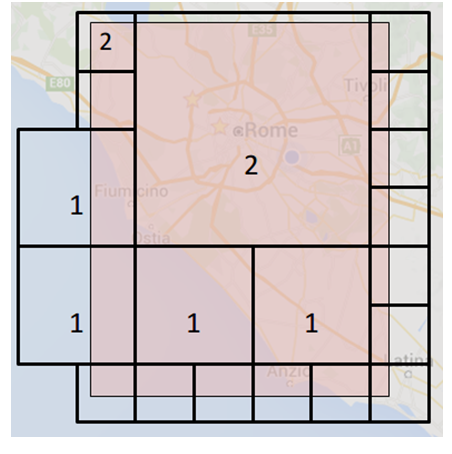}
		\label{f:constrained}
		
	}
	\caption{Range-query and tessellation approaches in case of grid indexing with three levels 0,1,2 and level-ratio 4}
	\label{f:indexing}
	
\end{figure*}

\section*{APPENDIX III - Tessellation Algorithm}
A range-query of an area $A$ is resolved with a set of tile-queries for tiles identified by the tessellation procedure. The set $T$ of tiles forming the tessellation covers an area $B$, which contains the area $A$, but also some additional border space, due the fact that the area $A$ may be not aligned with the grid (e.g., see fig. \ref{f:min-streatch-and-tiles}). We define \emph{tessellation stretch} $TeS$ the ratio between the area $B$ and the area $A$, namely $TeS = area(B)/area(A) \geq 1$.

A \emph{minimum stretch} tessellation is formed by the minimum set of the smallest tiles that intersects the area $A$, e.g. level-2 tiles as shown in fig. \ref{f:min-streatch}. However, this procedure may return many tiles, even for small values of $A$, which should be queried through ICN means, dramatically increasing the overall range-query time. For instance, using 1 km x 1 km tiles, a range query of 50 km x 50 km is tessellated at least with 2500 tiles, i.e. 2500 tile-queries are necessary to satisfy the range-query. Definitively too much.

To achieve a first reduction of the number of tiles, we can simply exploit the hierarchy of the grid, by removing each set of tiles of level-$n+1$ that completely fills the parent tile of level-$n$, and insert such a tile. This is for instance the case of the tessellation reported in fig. \ref{f:min-streatch-and-tiles}, in which a level-1 tile takes the place of 4 child level-2 tiles and, recursively, a level-0 tile replaces 4 child level-1 tiles.

\begin{figure}[t]
\centering
\includegraphics[scale=0.54]{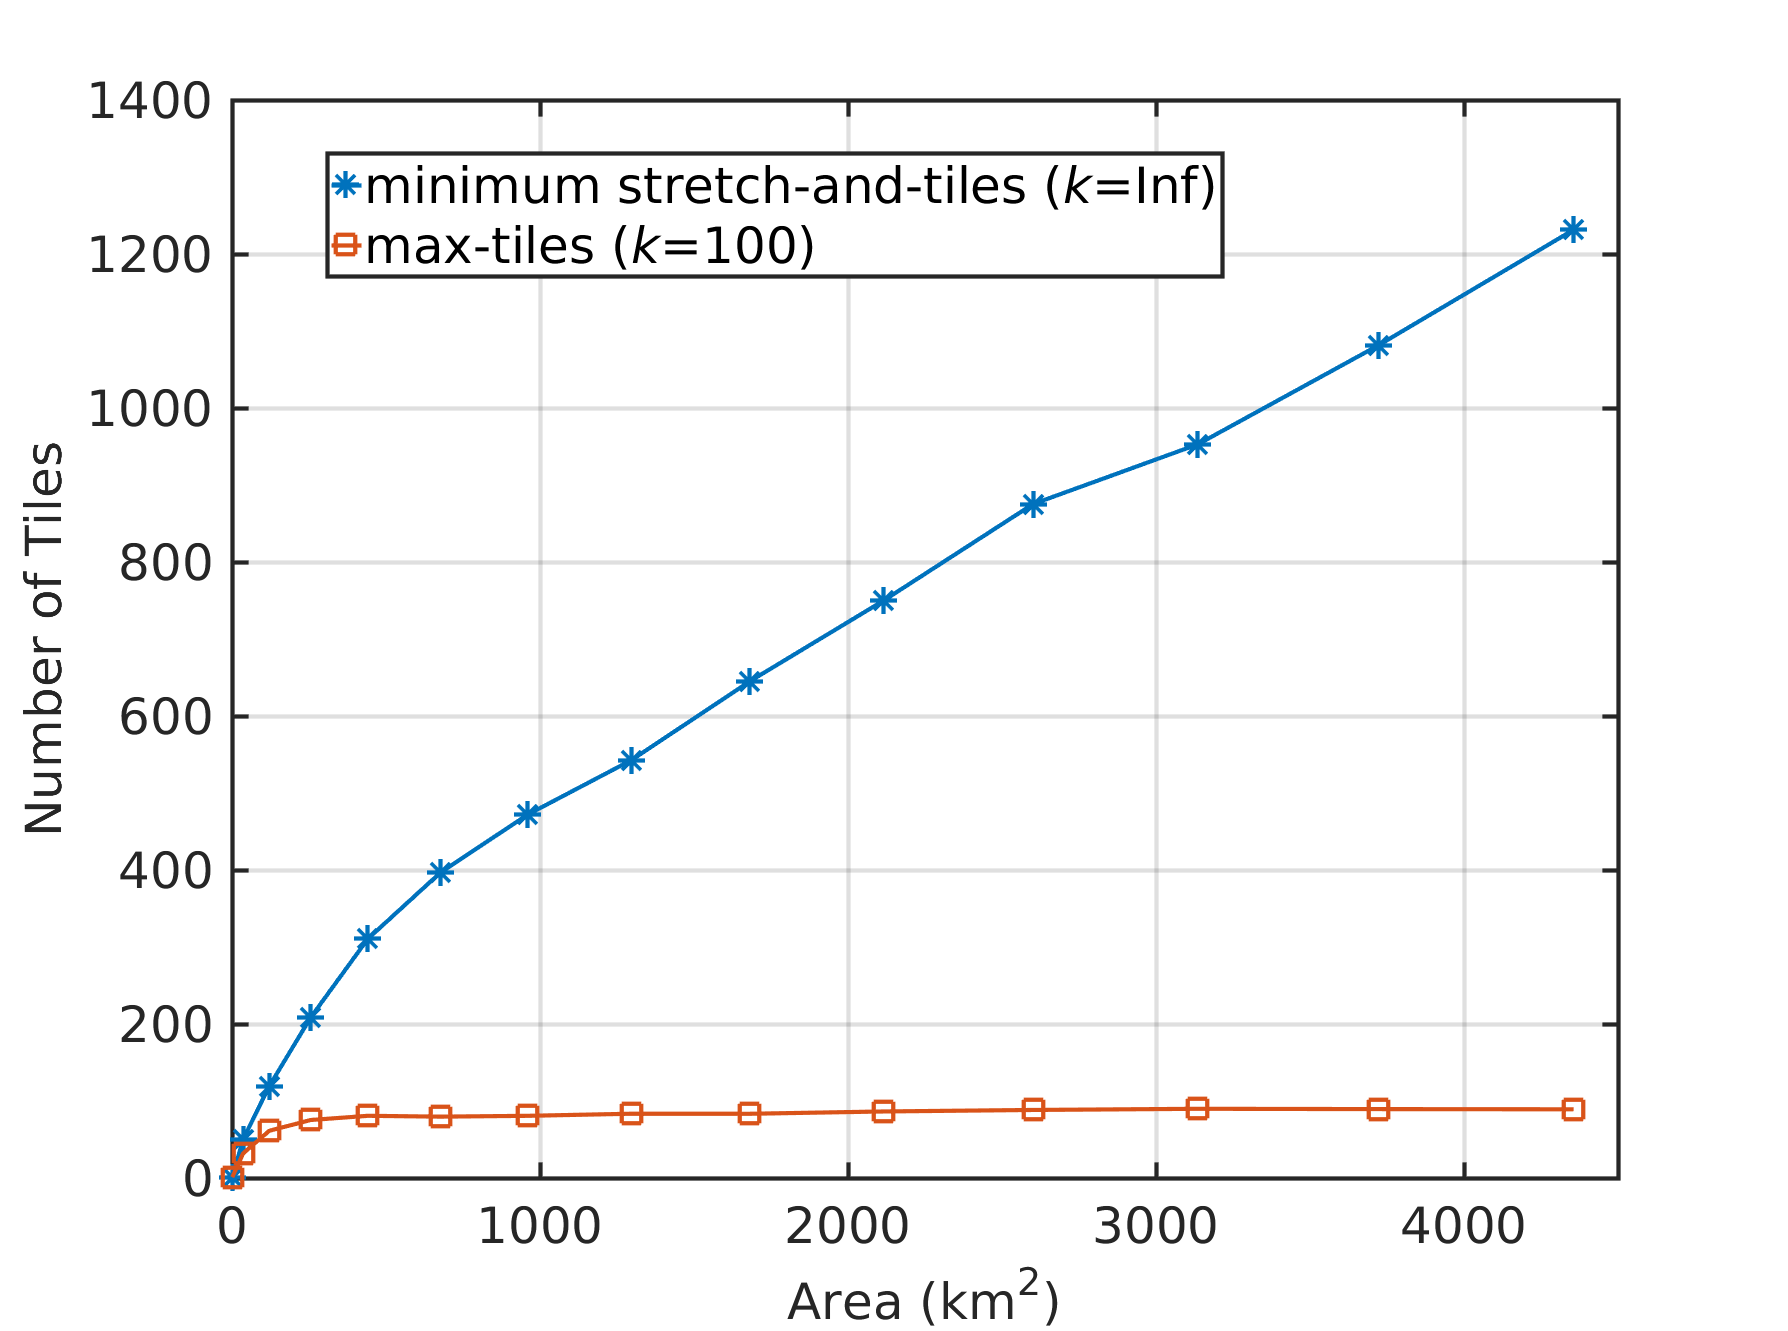}
\caption{Number of tiles vs. range-query area for minimal stretch-and-tiles tessellation for the OGB grid}
\label{f:tesseling-perf1}
\vspace{-8pt}
\end{figure}

However, even this \emph{minimum stretch-and-tiles} tessellation may return a high number of tiles, in case of large range-query, e.g. numbers of tiles greater than 500. Indeed, fig. \ref{f:tesseling-perf1} shows the number of tiles for randomly-centered range-query of square shape, whose area is the x-axis of the plot, by using the OpenGeoBase spatial grid. Such high values are usually due to the numerous small tiles used to fill the borders of the range-query area and/or to the misalignment of the range-query area with respect to the grid hierarchy. 

For this reason, we developed a \emph{constrained} tessellation algorithm, in which it is possible to fix the maximum number $k$ of returned tiles. For instance, fig. \ref{f:constrained} shows the result of a constrained tessellation for $k=19$. The drawback is that the lower the maximum number of allowed tiles, the higher the tessellation stretch. 

An optimal constrained tessellation algorithm should find the set of $k$ tiles providing the minimum stretch. This problem can be made equivalent to a minimal-weight size-constrained set cover problem. The set $S$ to be covered is formed by the set of the smallest tiles intersecting the area $A$; the universe $U$ is formed by these tiles and all their parent tiles up to level-0. The cost of a tile of $U$ is its \emph{tile-stretch}, i.e. the ratio between the tile area and the area of its intersection with the range-query area. 

In 2015 the authors of \cite{golab2015size} demonstrated that this problem is NP-hard. Thus, we devised the simple, but effective, greedy algorithm \ref{a:ct}, reported below, which follows a top-down approach, by first inserting the necessary bigger tiles and then, iteratively, the necessary smaller ones. A level-$i$ tile is necessary when completing the tessellation with all remaining level-$(i+1)$ tiles would not be able to respect the constraint $k$. Thus a level-$i$ "aggregation" is surely necessary. For very large range-query, it is not possible to respect the constraint, even by using all biggest tiles of level-0. In this case, the algorithm returns the set of covering level-0 tiles, even if it exceeds the constraint.

\begin{algorithm} [ht]
\caption{Constrained Tessellation}
\label{a:ct}
%{\fontsize{8}{10}
\begin{algorithmic}
\Statex $k$ = max number of tiles
\Statex $n$ = number of levels of the spatial grid
\Statex $S$ = whole indexing tree
\Statex $leaf(S)$ = leafs of S, i.e. tiles of the tessellation
\Statex $MST(S)$ = minimum stretch-and-tiles reduction of $S$
\Statex
%\Statex\textit{Tesseling}\

\Statex\textit{constraint violation exception}
\If {Using all level-0 tiles the number of tiles $> k$}

\Return the set of covering level-0 tiles

\EndIf
\Statex
\Statex $S=MST(S)$

\While{number of $leaf(S) > k$}

$i=0$

\While{$i \leq n$}
\If {(A new level-$i$ tile is necessary)}
\State Insert a new level-$i$ tile with min tile-stretch
\State Remove all its children
\State break
\EndIf

$i=i+1$

\EndWhile
\EndWhile\\		
\Return leaf(S) 
\end{algorithmic}
%}
\end{algorithm}

This algorithm is not optimal; however, we made some trials using a brute-force search of the optimal solution, and we found extremely rare cases in which our solution is not the minimum stretch one. In any case, finding the optimal constrained tessellation is not the aim of this paper, as we just wanted to design a working solution.

\begin{figure}[t]
\centering
\includegraphics[scale=0.54]{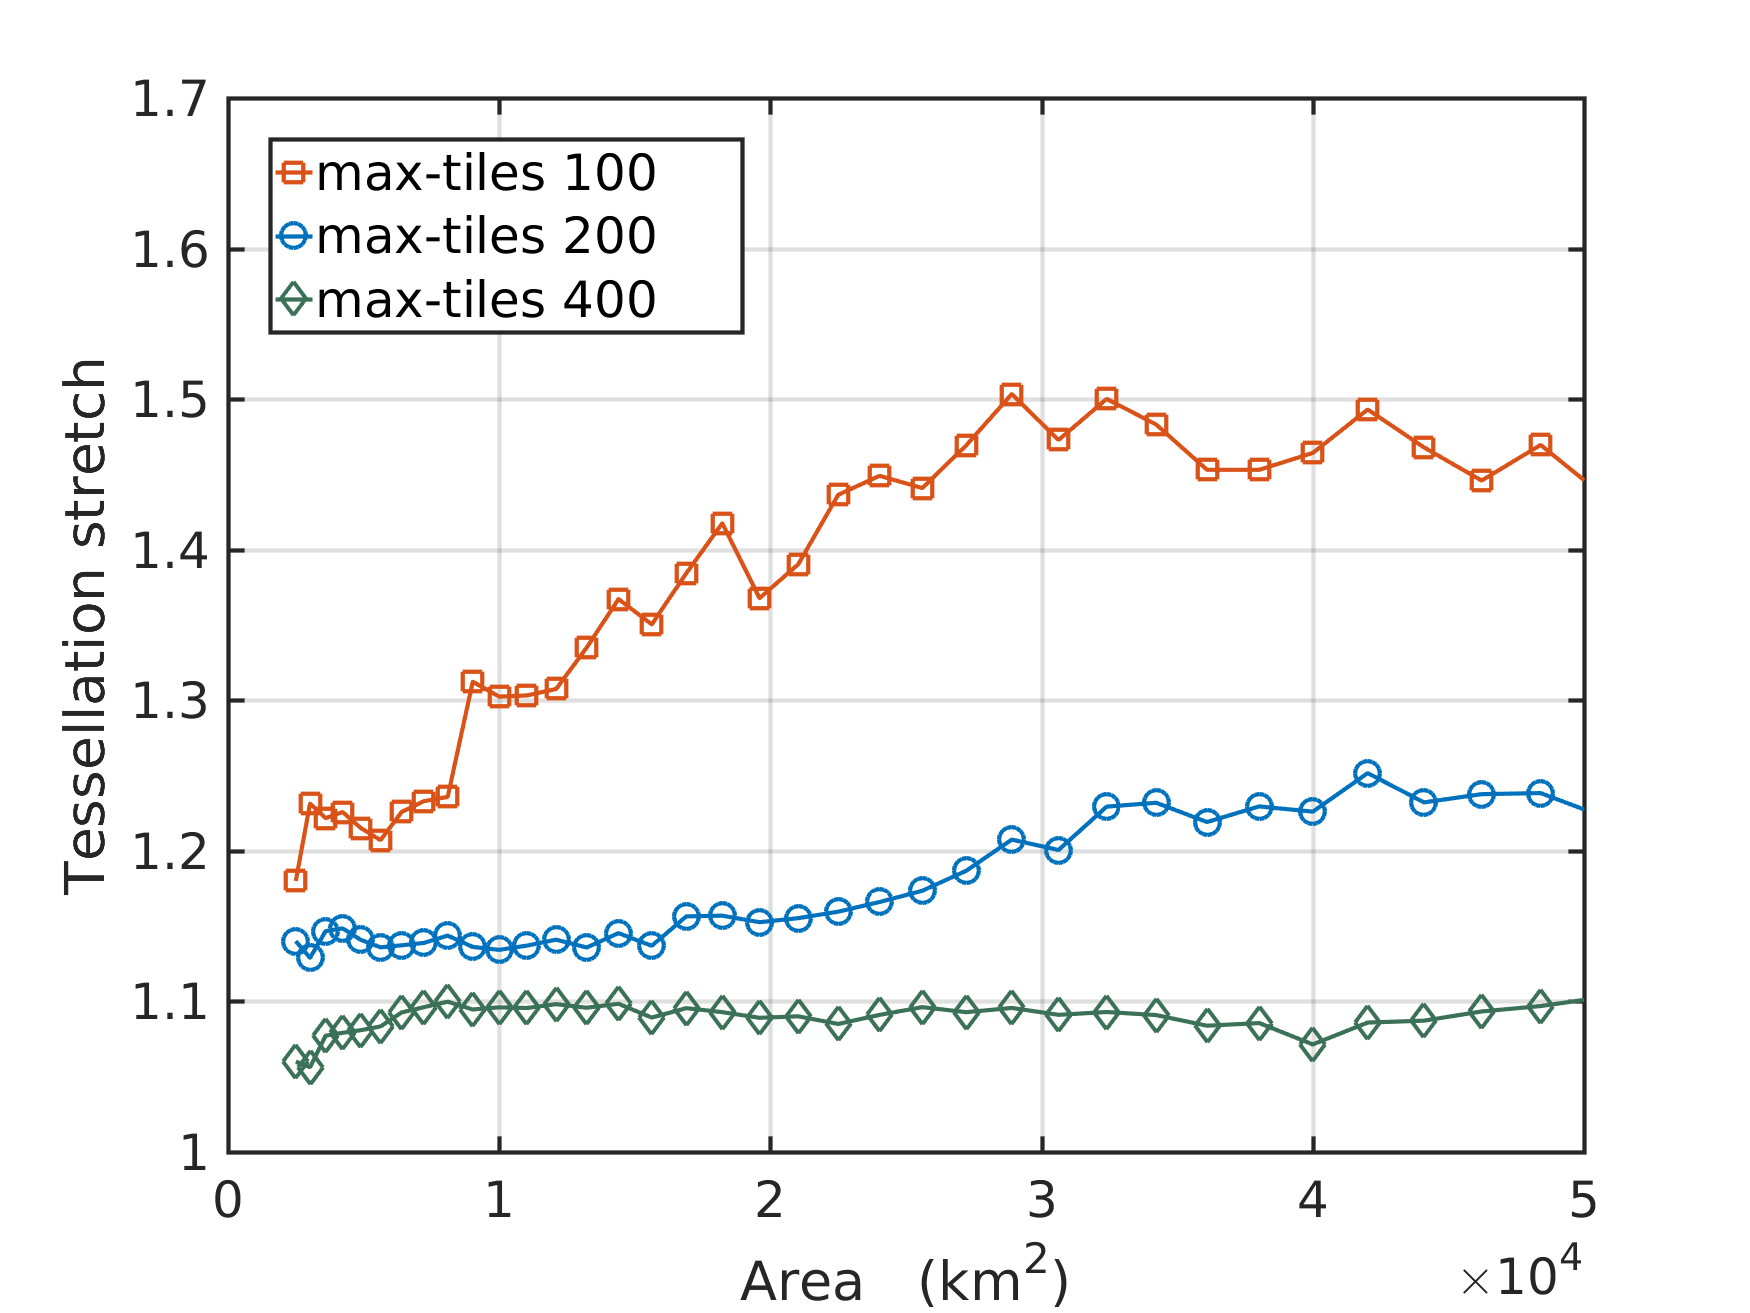}
\caption{Stretch of constrained tessellation vs. range-query area for the OGB spatial grid}
\label{f:tessellating-strech}
\vspace{-6pt}
\end{figure}

Fig. \ref{f:tesseling-perf1} shows that the constrained tessellation algorithm is actually able to reduce the number of queries up to the constraint $k=100$. Fig. \ref{f:tessellating-strech} reports the expected drawback: the increase of the tessellation stretch when the maximum number of tiles $k$ decreases. 
%Roughly, using 100 tiles we achieve have a stretch about of 50\% for very large query-areas, such as 50,000 km$^2$. Using 200 and 400 tiles this value fall down to 22\% and 10\%, respectively \footnote{We observe that also in case of the unconstrained minimal stretch-and-tiles solution there is a little stretch due to the fact that we can not have a resolution lower than the smaller grid level; however stretch value are extremely close to one}.     
With stretch greater than 1, a range-query returns geo-referenced information related to an area that is greater than the requested one, with a consequent increase of the network traffic. 
%which can be filtered out at the application end. 
Consequently, on the one hand, reducing the number of tiles accelerates the range-query processing time, since less ICN tile-queries are required; on the other hand, we are increasing the transmission time, since transferred data may increase. Clearly a trade-off is needed, which depends on the density and volume of geo-referenced information. Such values are application-dependent.
